# Supplementary material for: Tracking UWB Devices Through Radio Frequency Fingerprinting Is Possible
Source: arXiv:2501.04401 source file (2025-01-08)
Supplement: Supplementary file 1 [file appendix.tex]

\begin{appendices}

    \section{Technical Characteristics}

        All the measurements are made on devices that follows exactly the same hardware and software configuration. The technical specs of the experimental material is as follows:

     \begin{itemize}
         \item[-] Manufacturer: Qorvo (formerly, Decawave)
         \item[-] UWB Channel : 5 (6489.6 MHz center frequency)
         \item[-] Sampling frequency: ?
         \item[-] Options: STS mode ?, Header length ? 
         \item[-] UWB mode: HRP mode 
     \end{itemize}

\end{appendices}
